# Supplementary material for: Graphs of Edge-Intersecting Non-Splitting Paths in a Tree: Representations of Holes-Part II
Source: arXiv:1309.6471 source file (2018-01-09)
Supplement: Supplementary file 1 [file appendix.tex]

\newpage
\appendix

\noindent{{\Large \textbf{Appendices}}}
